# Supplementary material for: DAPPLE: A Pipelined Data Parallel Approach for Training Large Models
Source: arXiv:2007.01045 source file (2020-07-02)
Supplement: Supplementary file 1 [file appendix.tex]

\appendix

\subsection{Planning Formulation}
% test
\label{app:formulation}
\subsubsection{Preliminaries}
\label{sec:planner-preliminaries}
Throughout this section, we'll use the following set of consistent notations:

\subsubsection*{Planning Results}
\begin{itemize}
\setlength\itemsep{0.1em}
\item $L$: \textit{Batch Latency}, the time it takes to finish a single global
  batch
\item $Q$: Pivot stage, the stage we use to estimate $L$
\item $S$: Number of stages
\item $M$: Number of micro-batches
\item $\phi_s$: Initial amount of micro-batches injected to stage $s$
\item $g_s$: The GPU IDs allocated for stage $s$
\item $r_s$: The replication factor of stage $s$, $r_s = |g_s|$
\item $l_s$: The layer IDs allocated for stage $s$
\end{itemize}

\subsubsection*{Model Information}
\begin{itemize}
\setlength\itemsep{0.1em}
\item $N$: Number of layers in the model
\item $C$: \textit{Compute Times}, the total compute time of the model
  \begin{itemize}
  \item $C_s$: Compute times of stage $s$
  \item $C[i]$: Compute times of layer $i$
  \item $F_s$: Forward compute time of stage $s$
  \item $B_s$: Backward compute time of stage $s$
  \end{itemize}

\item $A$: \textit{Activation Size}, the total activation size of the model
  \begin{itemize}
  \item $A_s$: Output activation size of stage $s$
  \item $A[i]$: Activation size of layer $i$
  \end{itemize}

\item $P$: \textit{Parameter Size}, the total parameter size of the model
  \begin{itemize}
  \item $P_s$: Parameter size of stage $s$
  \item $P[i]$: Parameter size of layer $i$
  \end{itemize}
\end{itemize}

\subsubsection*{Environment}
\begin{itemize}
  \setlength\itemsep{0.1em}
  \item $G$: number of GPUs in the cluster
  \item $seps$: GPU distribution data, e.g. [8, 16] for 2 machines each with 8
    cards, and [8, 12] for two machines where the first one has 8 GPUs and the
    second has 4.
\end{itemize}
\subsubsection*{Helper Functions}
\begin{itemize}
\setlength\itemsep{0.1em}
\item $AR(size, gids)$: time to perform AllReduce with $size$ bytes of gradients
  between GPUs $gids$
\item $SC(size, g1, g2)$: time to perform \emph{Split-Concat} with $size$ bytes of
  activations from GPUs with ID $g1$ to GPUs $g2$
\end{itemize}

\subsubsection{Modeling the Pipeline Length}
\label{sec:planner-pipeline-length-modeling}

\subsubsection{Estimating $L$ for a Simplified Pipeline}

\begin{figure}[htbp]
  \centering
  \includegraphics[width=\linewidth]{./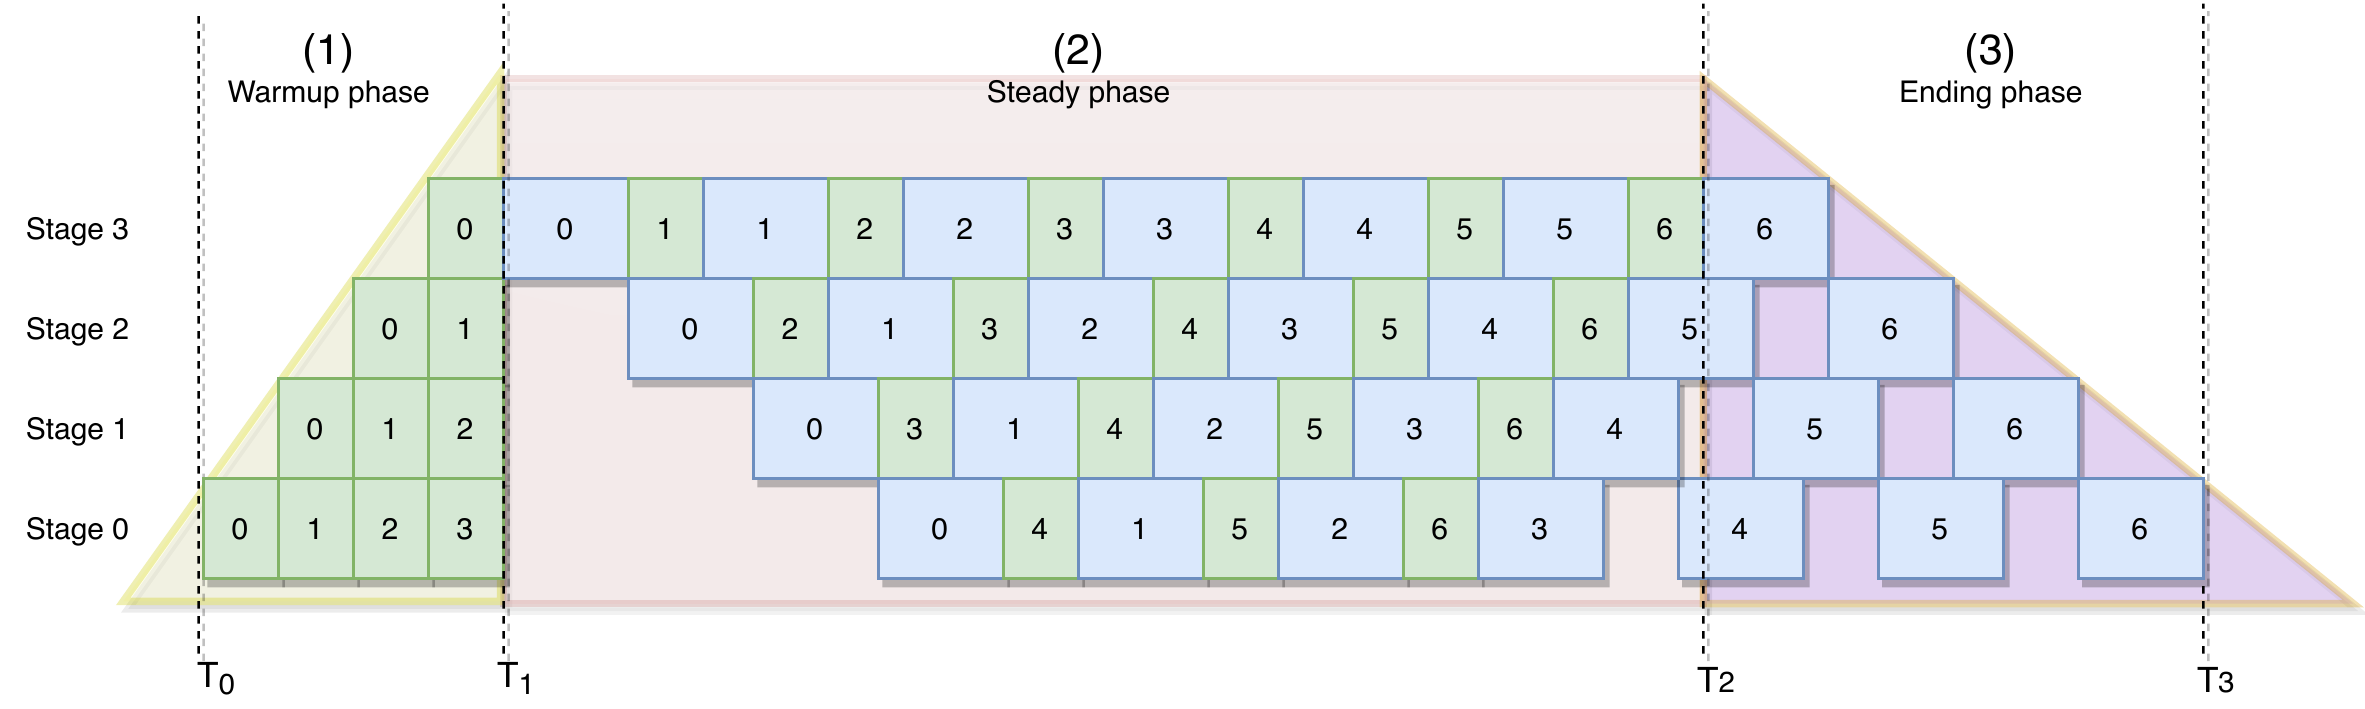}
  \caption{\label{fig:dapple-simple-pipeline}
    \emph{DAPPLE} simple pipeline.}
\end{figure}

Different from an asynchronous pipeline, in which a so-called "stable states"
can be achieved once the training process finishes the warm-up phase,
synchronous pipeline requires a synchronization barrier for each global batch to
do gradients aggregation. Therefore, a synchronous pipeline naturally forms a trapezoid.

Fig. \ref{fig:dapple-simple-pipeline} presents a simple pipeline where there
is no network overhead and the stages are split evenly. In order to estimate the
$L$ for this case, it makes sense to view the pipeline as three phases: (1)
Warmup phase, (2) Steady phase, and (3) Ending phase.

\textit{(1) Warmup phase}

The latency for the Warmup phase, indicated by the interval between $T_0$ and
$T_1$ in Fig. \ref{fig:dapple-simple-pipeline}, can be calculated by summing up all the
forward computation time:

\begin{equation}
  T_1-T_0 = \sum_{s=0}^{3} F_s
\end{equation}

\textit{(2) Steady phase}

In this evenly partitioned pipeline, the latency of the Steady phase is equal to
the time of 6 micro-batches in the topmost stage.

\begin{equation}
T_2-T_1 = (7-1) \times (F_3 + B_3)
\end{equation}

\textit{(3) Ending phase}

Ending phase can be calculated similarly to the Warmup phase:

\begin{equation}
  T_3-T_2 = \sum_{s=0}^{3} B_s
\end{equation}

Therefore, in this particular case, the batch latency $L$, from $T_0$ to $T_3$ in
the figure, can be written as:

\begin{equation}
  L = T_3-T_0 = \sum_{s=0}^{3} F_s + (7-1) \times (F_3 + B_3) + \sum_{s=0}^{3} B_s
\end{equation}

\subsubsection{Generalize to Non-uniform Pipelines}

In the previous Fig. \ref{fig:dapple-simple-pipeline}, we had the
simplification that the pipeline is partitioned evenly, i.e. the computation
blocks in each stage are equal.

\begin{figure}[t]
  \centering
  \includegraphics[width=\linewidth]{./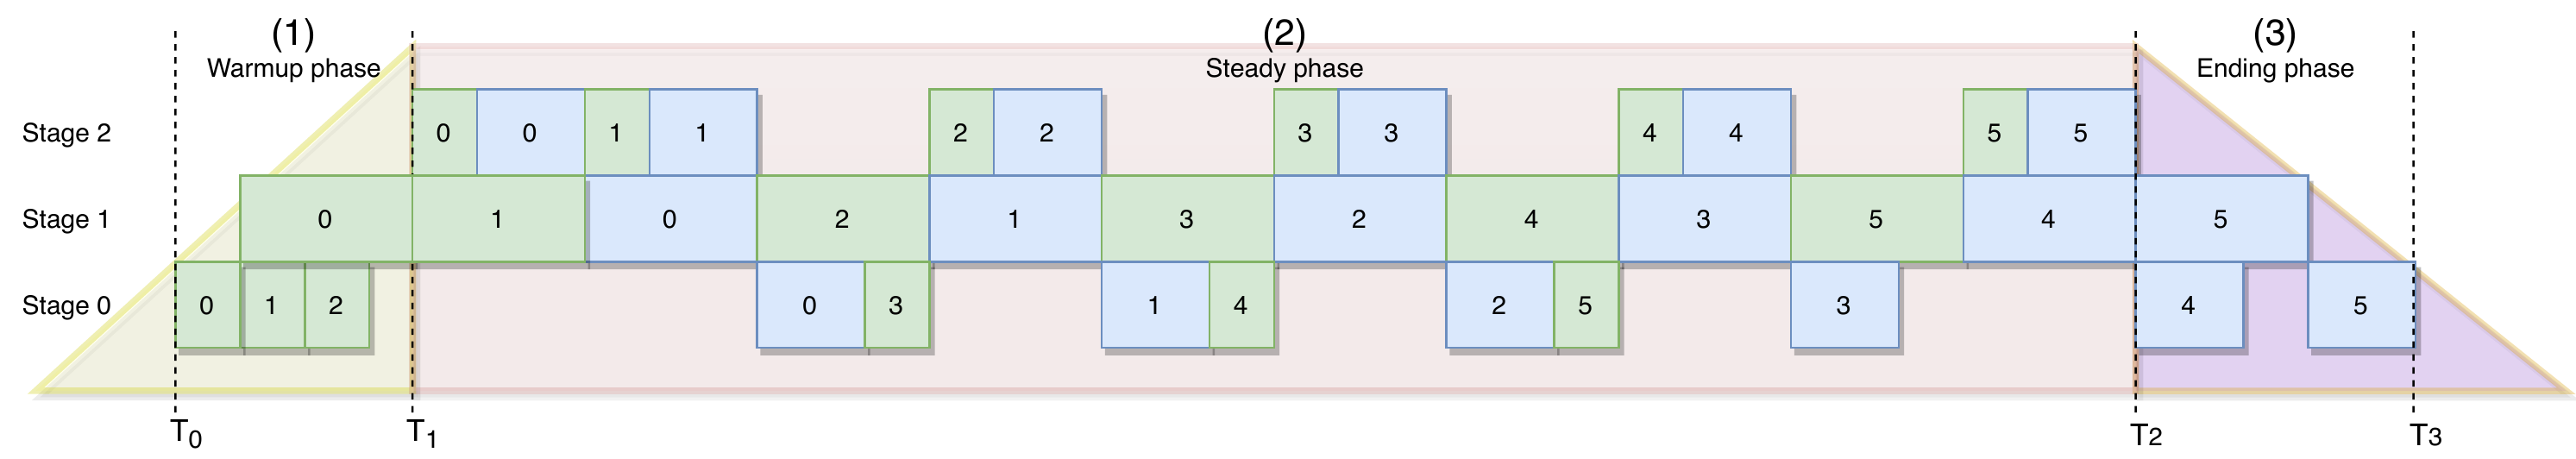}
  \caption{\label{fig:dapple-unbalanced-pipeline}
    \emph{DAPPLE} unbalanced pipeline example.}
\end{figure}

Consider the following unbalanced pipeline in Fig.
\ref{fig:dapple-unbalanced-pipeline}. The calculation for $L$ from the previous
equation no longer works since (1) the latency of the warmup phase is not equal
to the sum of forward computations of all stages, (2) the latency of the steady
phase cannot be estimated by time of micro-batches from the topmost stage, and
(3) the latency of the ending phase is not equal to the sum of backward
computations of all stages.

Therefore here we introduce a new concept: \emph{Pivot Stage} $Q$. In our
previous simplified pipeline, $Q$ is the topmost stage. The latency of the
warmup phase can be viewed as the sum of forward computations from stage 0 to
stage $Q$, and similar generalization can be applied to the ending phase. For
the steady phase, instead of using the topmost stage time for latency
estimation, we now depend on the forward/backward time of stage $Q$. The
equation (4) can then be rewritten as:

\begin{equation}
  L = T_3-T_0 = \sum_{s=0}^{Q} F_s + (M-1) \times (F_Q + B_Q) + \sum_{s=0}^{Q} B_s
\end{equation}

where $Q = 3$ for the case in Fig. \ref{fig:dapple-simple-pipeline}.

For an unbalanced pipeline shown in Fig. \ref{fig:dapple-unbalanced-pipeline},
we now simply take the stage with the longest forward+backward time as the pivot
stage $Q$, i.e. $Q = \arg \max_{s=0}^{S} (F_s + B_s)$. By plugging $Q=1$ in this
case, we get a correct estimation of the pipeline latency.

\subsubsection{Batch Length Estimation with Network}
\label{sec:planner-ble}
In real world scenarios, network effects are usually not negligible. And we take
that into consideration by arranging cross-stage communication as a separate
stage in the pipeline, and by putting gradients aggregation to the back of the
corresponding stage to maximize the overlap with computation. An example DAPPLE
pipeline is presented in Fig. \ref{fig:HPGO-Pipeline}.

\begin{figure*}
  \centering
  \includegraphics[width=\linewidth]{./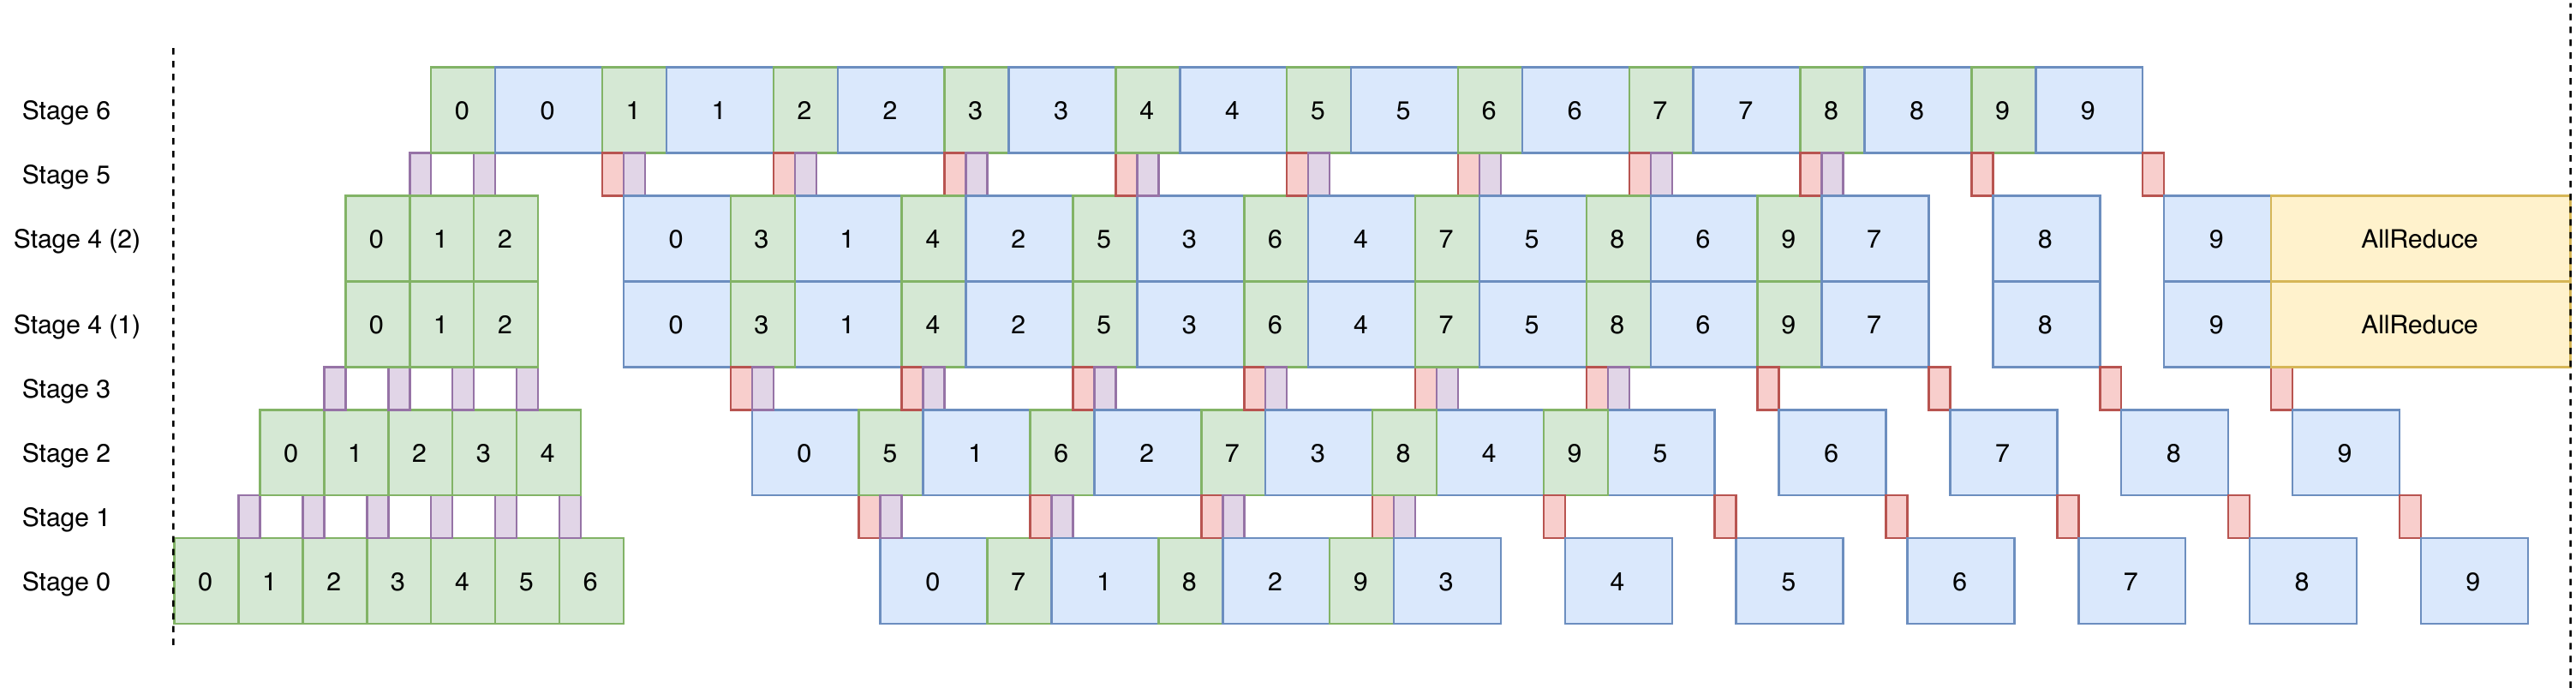}
  \caption{\label{fig:HPGO-Pipeline}
    \emph{DAPPLE} Pipeline example.}
\end{figure*}

\emph{1. Cross-stage Activation Communication with Split-Concat}

\begin{figure}[htbp]
  \centering
  \includegraphics[width=.9\linewidth]{./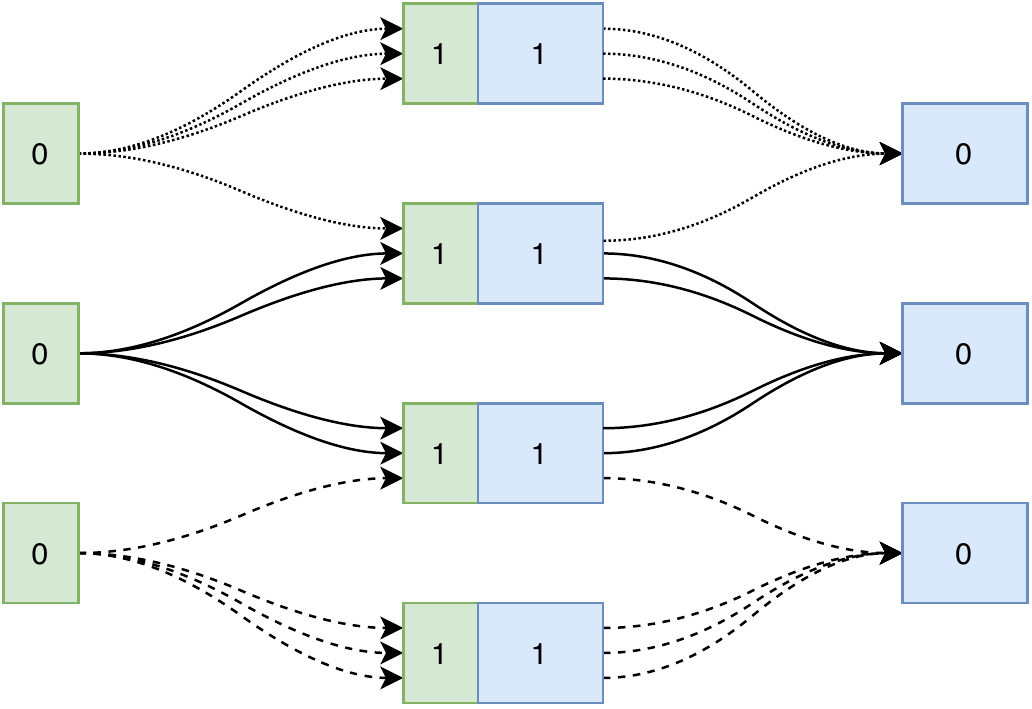}
  \caption{\label{fig:HPGO-SplitConcat}
    Split-Concat transfer.}
\end{figure}

As shown in Fig. \ref{fig:HPGO-SplitConcat}, our SplitConcat scheme ensures
the output activation from the previous stage is evenly split for the next
stage, and the activation transfer is done in a \emph{first-come-first-served}
way to alleviate the impact of straggler GPUs.

In the planner, we model the communication by firstly aggregating all the
activations with the same source and destinations, and bounding the
communication time by the slowest portion of those communication streams.

As mentioned in the preliminaries \ref{sec:planner-preliminaries}, we use
$SC(size, g1, g2)$ to refer to the time it takes to transfer $size$ bytes of
activations from $g1$ to $g2$. We put the activation communication as a separate
stage in the pipeline by defining a new stage $s$ between every two
computational stages $s-1$ and $s+1$, and set its $F$ and $B$ to be $F_s = B_s =
SC(A_s, g_{s-1}, g_{s+1})$.

% The estimation method still applies after adding network communications as
% separate stages, 

\emph{2. Parameter Updates with AllReduce}
The AllReduce operation is only needed for those stages with more than one
replication, and it can be performed immediately after the last backward block
of the corresponding stage, or even partially overlapped with the last backward
block.

For the Warmup phase and Steady phase, the previous calculation methods still
apply, but for the ending phase, since we could have potentially a very long
AllReduce, we now check for the max potential latency of that phase for each
stage:

\begin{equation}
  T_3 - T_2 =  + \max_{s=0}^{S}
  \left\{
    \begin{array}{lr}
      -\sum_{a=Q}^s B_a + AR(P_s, g_s), & s > Q \\
      \sum_{a=s}^Q B_a + AR(P_s, g_s), & s \le Q
    \end{array}
  \right.
\end{equation}

And therefore the final equation for estimating the batch length $L$ with
network effects taken into account is as follows:

\begin{equation}
  Q = \arg \max_{s=0}^{S} (F_s + B_s) 
\end{equation}
\begin{equation}
	\begin{split}
    L & = \sum_{s=0}^{Q} F_s + (M-1) \times (F_Q + B_Q)  \\
    & + \max_{s=0}^{S} \Bigg( (s > Q ? -\sum_{a=Q}^s B_a : \sum_{a=s}^Q B_a) + AR(P_s, g_s) \Bigg)
  \end{split}
\end{equation}

\subsubsection{Selecting the best $Q$}
\label{sec:planner-best-q}
In our previous calculations, the pivot stage $Q$ is selected to be the one with
the largest $F+B$ value, the ``busiest'' stage so to speak. In most cases, the
``busiest'' stage usually has the lowest bubble overhead, allowing us to
accurately estimate the latency of the steady phase by $(M-1) \times (F_Q+B_Q)$.

However, the estimation can be off by a fair amount if $Q$ is not the topmost
stage, therefore we propose a more robust way to determine the pivot stage $Q$.

Initially set $Q$ to the topmost stage: $Q = S-1$, and whenever we explore a new
lower stage $t$, we check if stage $t$ is ``busier'' than $Q$ using the
following condition:

\begin{equation}
  \begin{split}
    Q' & = \arg \max_{s=Q-1}^t \max \\
      & \Big( (M-1) \times (F_Q+B_Q) + \sum_{s'=Q}^s (F_{s'}+B_{s'}) \\
      & , (M-1) \times (F_s + B_s)\Big)
  \end{split}
\end{equation}

This essentially still checks for the ``busiest'' stage, but instead use the
following heuristics:

The bottom stage $s-1$ has a larger inner bubble overhead if $(M-1) \times
(F_{s-1}+B_{s-1}) < M \times (F_s+B_s)$.

As shown in Fig. \ref{fig:HPGO-Pipeline-Select-Q}, we check if $M-1$
micro-batches in the current stage exceeds the bound between the two dotted
vertical line. If it does, then the stage $Q$ will have bubbles within
the stage, and in such case we update $Q$ to be the current stage $t$.

\begin{figure}[htbp]
  \centering
  \includegraphics[width=\linewidth]{./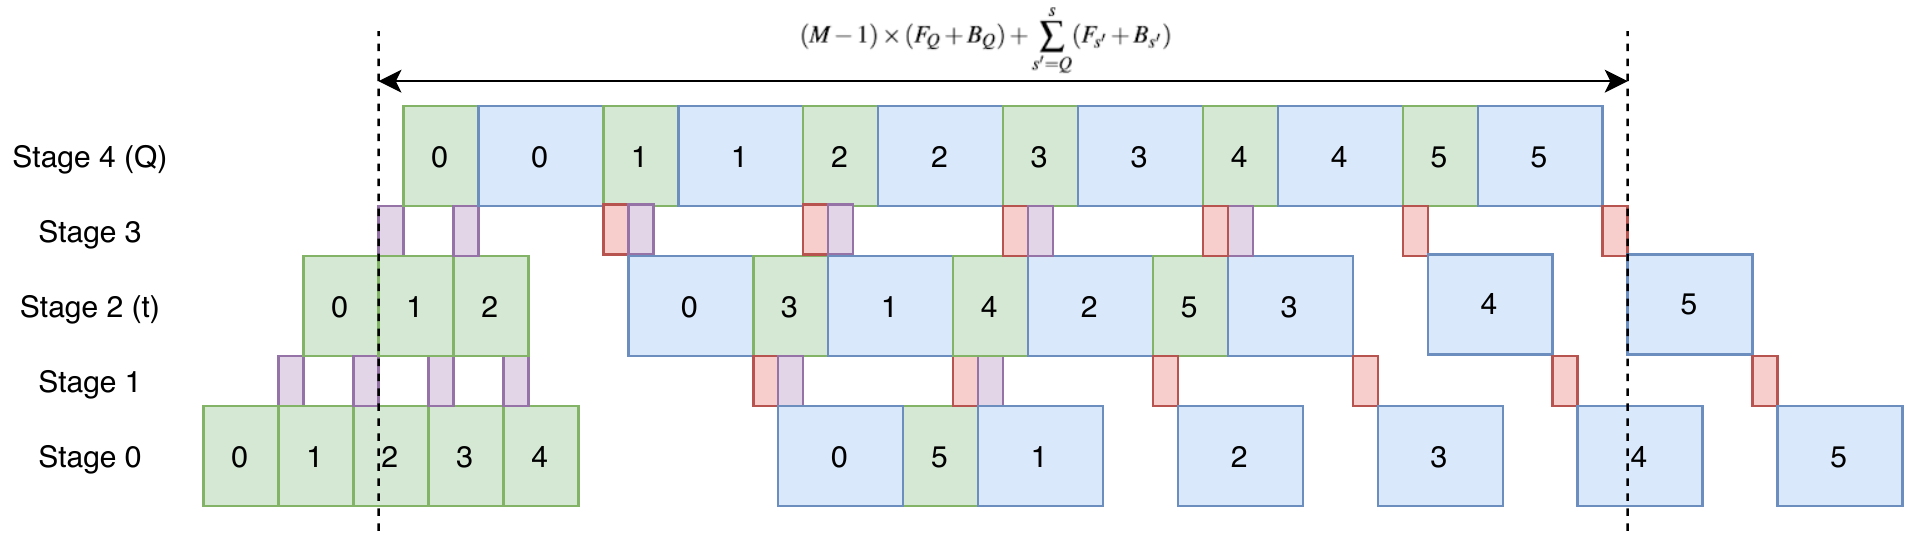}
  \caption{\label{fig:HPGO-Pipeline-Select-Q}
    Checking stage t with Q.}
\end{figure}

Although still not accurate enough in some corner cases, it has been proven to
be accurate enough to act as a value function for our planning algorithm.

\subsubsection{Accurate Calculation of the Batch Length}
\label{sec:planner-recursive-calculation}

To calculate the latency of a global batch even more accurately, we use a double
recursion method to simulate the DAPPLE micro-batch arrangement.

We use $f[i, x]$ to denote the forward block for micro-batch $\#i$ at stage $x$,
and $f[i, x].s$ and $f[i, x].e$ for the start and end time for that block
respectively. A \textit{Forward Block} can be either Forward Evalution
computation or upward communication to higher stages. We use $b[i, x]$ similarly
for backward blocks. We use $\phi[x]$ to denote the number of micro-batches to
inject to stage $x$ initially before performing the 1F1B arrangement.

\textit{Forward Constraints}: For forward blocks, each block $f[i, x]$ has to
satisfy the following three conditions:
\begin{enumerate}
  \item it has to be performed after the forward block for the previous
    micro-batch
  \item it has to be performed after the forward block from lower stages 
  \item it has to be performed after the backward block of certain micro-batch
    in order to fulfill the requirements of our 1F1B arrangement.
    
\end{enumerate}

Therefore, we have the following formula for an arbitrary forward block:

\begin{equation}
	f[i, x].s = \max
      \left\{
        \begin{array}{lr}
          b[i - \phi[x], x].e & \\
          f[i-1, x].e & \\
          f[i, x-1].e &
        \end{array}
      \right.
\end{equation}

\begin{equation}
	f[i, x].e = f[i, x].s + F[x]
\end{equation}

\textit{Backward Constraints}: for backward blocks, we have three similar constraints:
\begin{enumerate}
  \item it has to be performed after the backward block for the previous
    micro-batch
  \item it has to be performed after the backward block from upper stages 
  \item it has to be performed after the forward block of certain micro-batch in
    order to fulfill the requirements of our 1F1B arrangement.
\end{enumerate}

\begin{equation}
	b[i, x].s = \max
      \left\{
        \begin{array}{lr}
          f[i + \phi[x] - 1, x].e & \\
          b[i-1, x].e & \\
          b[i, x+1].e &
        \end{array}
      \right.
\end{equation}

\begin{equation}
	b[i, x].e = b[i, x].s + B[x]
\end{equation}

\textit{Batch Latency}: We use a similar approach as our analytical estimation
above to calculate the batch latency. For every stages, we add the AllReduce
time to the end of the backward block of the last micro-batch, and calculate the
maximum amongst all stages.

\begin{equation}
	PL = \max_{x=0}^{S} {\Biggl(b[m, x].e + AllReduce[x] \Biggr)}
\end{equation}

This calculation of batch latency, despite taking $O(M \times S)$ time
complexity, is more accurate than the estimation method above, and can be used
to further reduce the latency by exploring various micro-batch arrangements.

\subsection{Empirical Validation of Approximation Accuracy}
\label{sec:planner-empirical-analysis}
In practice, we will use the estimation method mentioned above
\ref{sec:planner-ble} rather than the accurate recursive one to rank all the
potential planning results, and will use the accurate result while outputing the
theoretical speedup of the planning solution. To this end, we need to assess the
bound between the accurate result of $L$ and our estimated one.

% plan中间为什么只需要相对顺序对就行
During the planning process, the batch latency $L$ is used as an optimization
objective to be minimized, and in the end we would output the plan that yields
the shortest batch latency. Therefore, we care much less about whether our
estimated $L$ is close enough to the accurate one, but more about whether the
relative ordering of the results from these two methods matches up. We could
tolerate a huge margin of error for our estimation, and as long as the relative
ordering is correct, we would still be able to get the correct planning results.

We set up an experiment to evaluate the accuracy of ranking pipeline latency. By
keeping the total compute time constant, we generate two random pipeline plan,
$A$ and $B$, each with three stages, denoting $[A_1, A_2, A_3]$ and $[B_1, B_2,
B_3]$, where $$A_1+A_2+A_3 = B_1+B_2+B_3$$

Since they can be viewed as two independent partitioning results of the same
model, we can estimate the batch length of the two with our analytical methods
\ref{sec:planner-ble}, and would get $A_{estimated}$ and $B_{estimated}$.
Similarly we calculate $A_{accurate}$ and $B_{accurate}$ with our recursive
method \ref{sec:planner-recursive-calculation}.

We then compare the relative latency of these two pipelines, and would consider
a comparison as a ``bad case'' for our estimation method only if: $$(A_{accurate}
- B_{accurate}) \times (A_{estimated} - B_{estimated}) < 0$$. In other words,
this is the case where our estimation method gives the wrong rank and could
potentially cause the planner to miss the optimal solution in our solution space.

We ran the experiments of pipeline ranking for 10 billion pairs of random
pipelines of the same model, with $M$ set to 16 and $\phi = [5,3,1]$, and got
$1204$ ranking errors out of $100000000$ attempts, which means that even if our
estimation might be off in some cases, it gives out the correct ordering most of
the time, with an error rate of $0.001\%$.

\subsection{Runtime Analysis}
The planning algorithm without device assignments takes \(O(N^4 \times M^2)\),
in which there are \(O(MN)\) sub-problem, with each one taking \(O(N^3*M)\).
This on its own can handle planning for flat network configurations.

With Device Placement turned on, the complexity increases by an exponential
factor due to enumeration of next available sets of GPUs for each iteration.
This would take an overall complexity of \(O(N^4 \times M^2 \times BF)\), where
\(BF = O(2^N)\) and in practice \(BF << 2^N\). 

\subsection{Insights from planning results}
\label{sec:planner-result-insights}

\subsubsection{\textbf{Number of stages v.s. Evenness}}
\label{sec:planner-num-of-stages}

For every model, we might have different ways to partition the model in which
every partition, when assigned to a proper numbers of GPUs, takes roughly the
same amount of time to complete. In this case, we have the conclusion that the
fewer stages we have in the pipeline, the higher its pipeline efficiency.

Suppose we have a 16-layer model with the same computation requirement for each
layer. The total compute time denoted as $C$ and the time for exchanging
activations and model weights are negligible. And we want to plan for the best
hybrid parallelism solution for a 2-machine cluster, with 8 GPUs on each node.

If the model is partitioned evenly, we can calculate the pipeline length as:
$$L = (m-1) \times C[top] + C$$
where $m$ corresponds to the number of micro-batches injected into the pipeline,
and $C$ the compute times array for the model in which each element $C[i], 0 \le
i \textless 16 $ corresponds to the compute time of each layer. $C[top]$ stands
for the computational time for the topmost stage, i.e. $C[top] = \sum_{i \in
  top} {C[i]}$.

Consider two possible solutions for splitting the model evenly and pipelining
all the partitions of the model:

\begin{enumerate}
	\item partition the model into 16 stages, i.e. one layer per stage
	\item partition the model into 2 stages, with 8 outer DP replications
\end{enumerate}

Since we effectively have 8 pipelines for solution 2, the micro-batch count for
each pipelines of solution 2 $m_2$ is equal to $\frac{1}{8} m_1$.

The length for solution 2 (DAPPLE) can be calculated as:

\begin{equation}
	\begin{split}
		L_2 & = (m_2 - 1) \times {\frac{1}{2} C} + C \\
			& = C \times (\frac{m_2}{2} + \frac{1}{2})
	\end{split}
\end{equation}

And the length of solution 1 (Pipeline):

\begin{equation}
	\begin{split}
		L_1 & = (m_1 - 1) \times {\frac{1}{16} C} + C \\
			& = (8 \times m_2 - 1) \times \frac{1}{16} C + C \\
			& = C \times (\frac{m_2}{2} + \frac{15}{16}) \\
			& > L_2
	\end{split}
\end{equation}

Notice that even if both solutions have the model perfectly partitioned,
\textbf{less stages in the pipeline leads to higher overall hybrid parallel
  efficiency}.

\subsubsection{\textbf{Intentional unevenness v.s. Evenness}}
\label{sec:planner-unevenness}

\begin{figure*}
  \centering
  \includegraphics[width=\linewidth]{./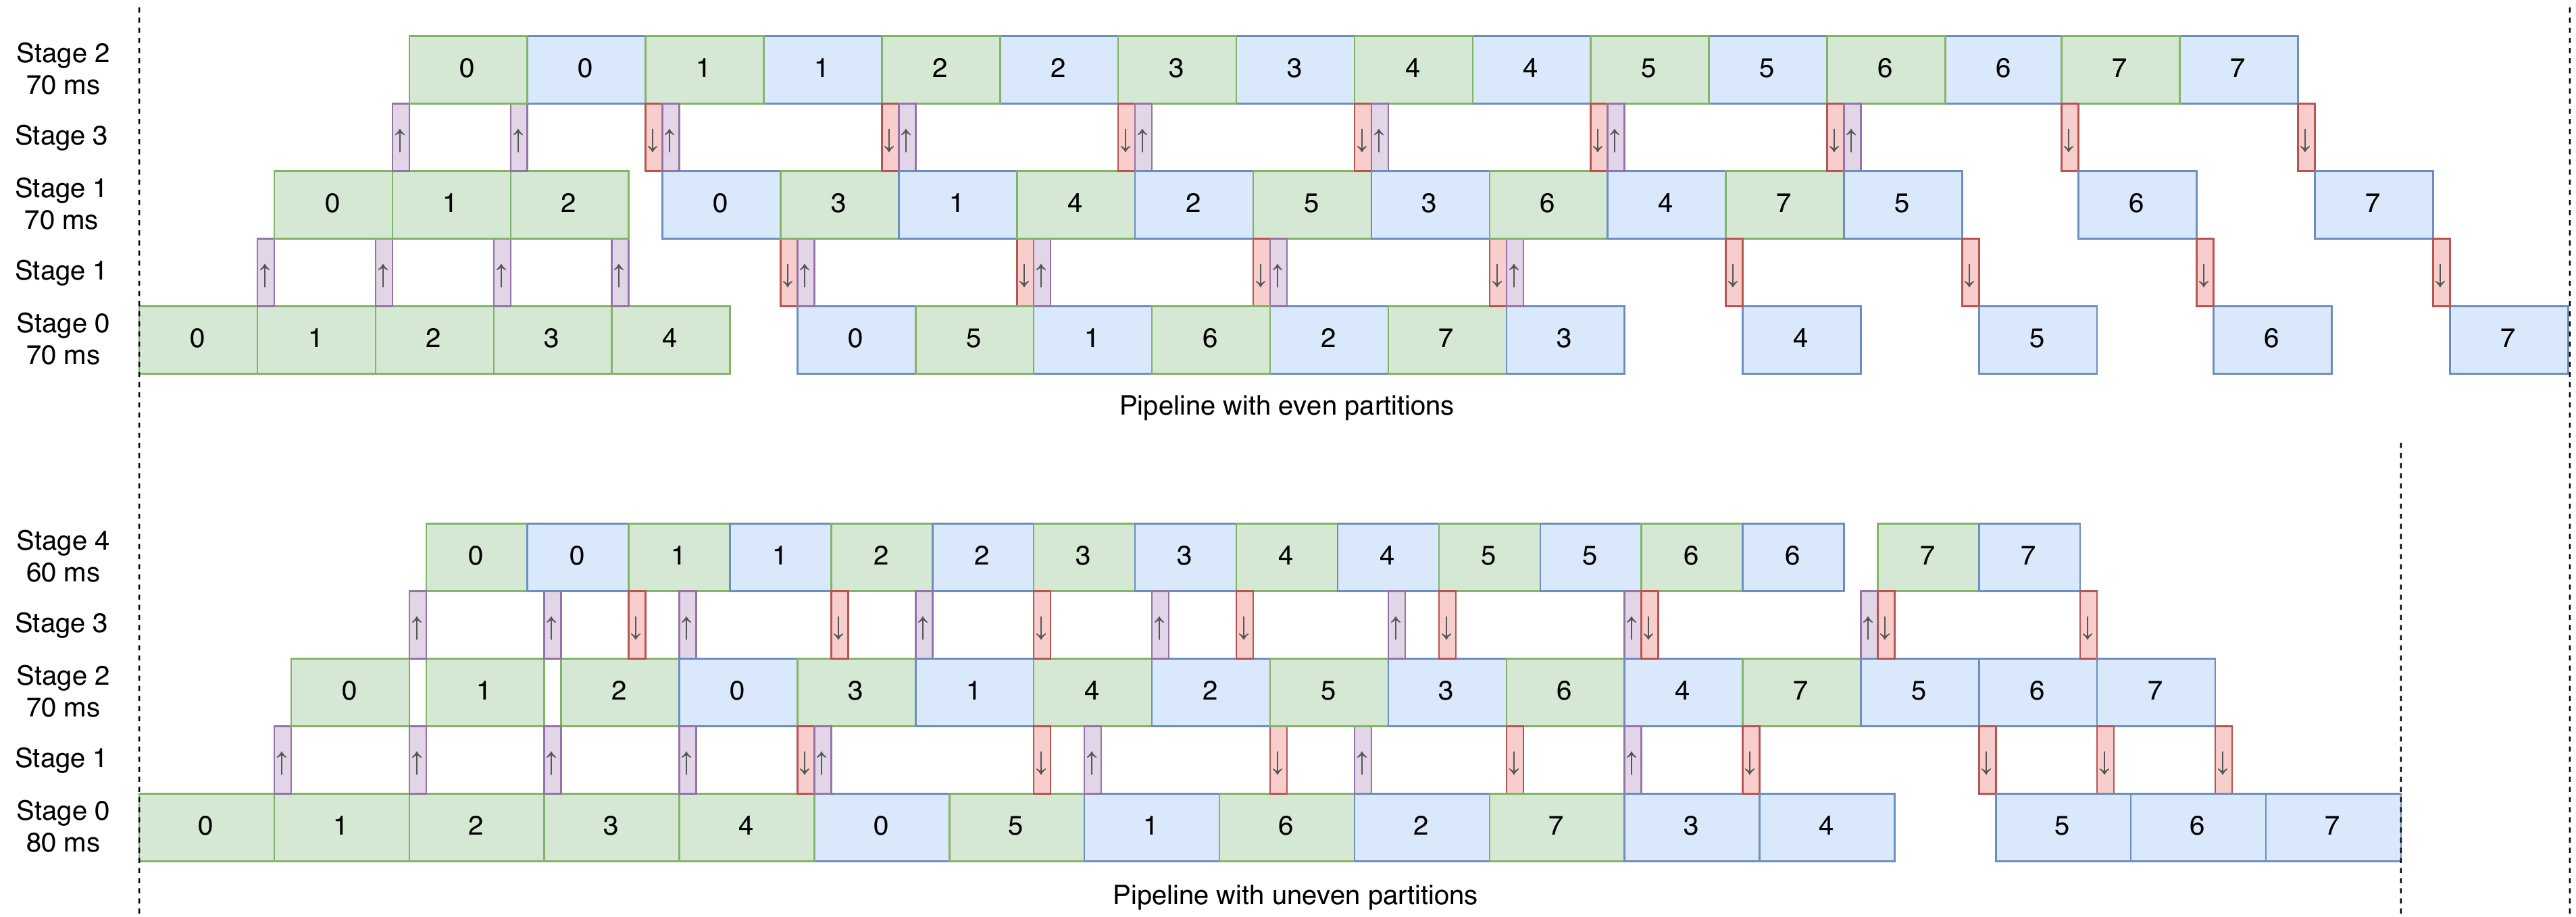}
  \caption{\label{fig:HPGO-Uneven-Pipeline}
    Uneven Pipeline Example.}
\end{figure*}

Although asynchronous hybrid parallelism might benefit from an even partitioning
policy, we found uneven pipelines yield higher performance under synchronous
training.

\textit{(1) Rightmost upper-triangular region for AllReduce} \\
As shown in Fig. \ref{fig:DAPPLE-Planning-Pipeline}, synchronous pipeline
naturally forms a trapezoid, and the rightmost triangular region can be used to
overlap current stage AllReduce operation with next stage backward computations.
Therefore an evenly partitioned pipeline could suffer from overly time consuming
AllReduce from the bottom stages. And instead we should aim for putting more
parameters into stages higher up, and decrease the weights for the bottom
stages.

\textit{(2) Allocate computation in increasing amount to minimize bubble overhead} \\
We also observed that if a pipeline is partitioned such that the compute time
from top to bottom is increasing, the pipeline effective time can be further
reduced. To be more specific, we can express this condition for stage $s$ and
$s-1$ as
$$C_s \times (m - 1)<= C_{s-1} \times (m - 1) <= C_s \times m$$

% NOTE: mb -> m, for number of micro-batches
% \added[id=muzhuo.yj]{Should we add the notation of mb here?}
The end-to-end time improvements can be seen in Fig.
\ref{fig:HPGO-Uneven-Pipeline}, where there is a clear performance advantage for model partitioned as 8:7:6 versus an even partition of 1:1:1. And as shown in the figure, this partitioning improvements is specific to our micro-batch scheduling
policy, and could cause performance regression on GPipe's micro-batch arrangement.

\subsubsection{\textbf{Same Partitioning, Different Micro-Batch Arrangement}}
\label{sec:planner-arrangement}

As previously stated in Section \ref{section:micro-batch-schedule}, we typically
use Policy A ($\phi = [1,1,2,2,3]$) when ACR is small, and policy B ($\phi =
[1,2,3,4,5]$) when the communication overhead is no longer negligible.

This is a heuristic we use to minimize the impact of inter-stage communication.
And in fact for every pipeline arrangement, we can find an optimal $\phi$ array
to maximize the training performance. Using a similar formulation as the one
presented in Section \ref{sec:planner-empirical-analysis}, we can again explore
different $\phi$ options on the same planning result, and select an optimal one.
In practice, our Planner output an additional result of the optimal $\phi$
alongside the hybrid parallelism plan.

In our empirical analysis, we found out that the optimal $\phi$ depends on
the latency distribution of the pipeline planning results, and the $\phi =
[1,2,3,4,5]$, although not always the optimal, yields best average performance
overall throughout all our experiments.
